# Supplementary material for: An analytical model of iceberg drift
Source: arXiv:1610.06403 source file (2016-10-20)
Supplement: Supplementary file 1 [file WagnerDellEisenman_SI_arXiv.pdf]

# Supplementary Information

## “An analytical model of iceberg drift”

BY TILL J.W. WAGNER, REBECCA W. DELL, AND IAN EISENMAN

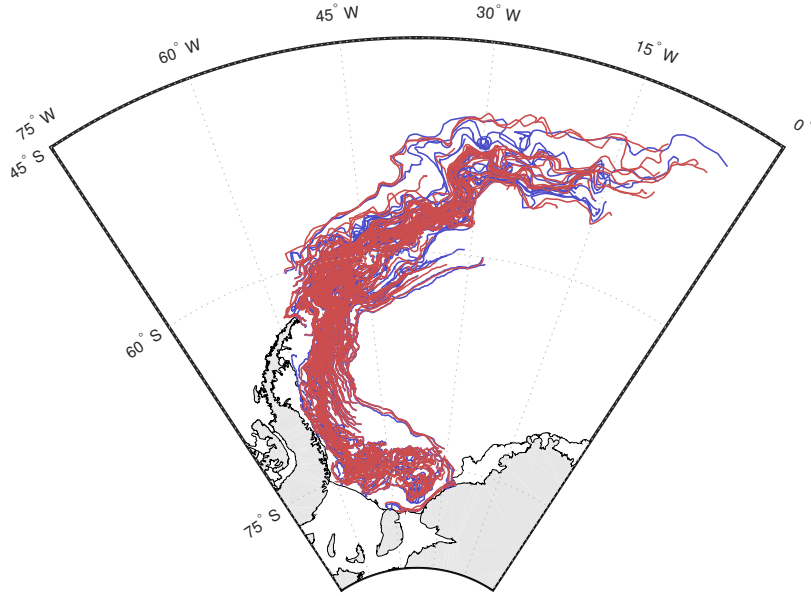

Figure S1. Antarctic iceberg trajectories for 200 large icebergs simulated using the analytical solution (6) with  $Md\vec{v}_i/dt = 0$  (red), as well as solving the model without calling on assumption 1 (blue).

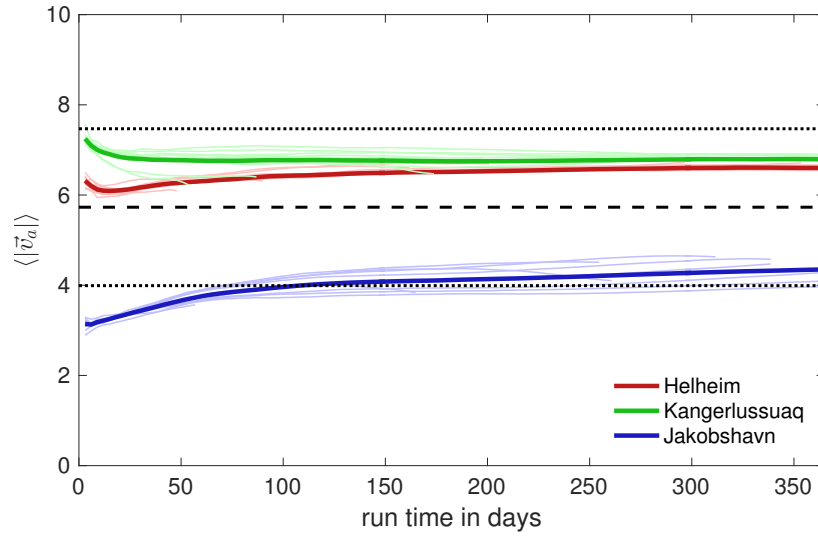

Figure S2. Evolution of 10m-surface wind velocities experienced by modeled icebergs plotted versus iceberg age (since inception). The faint lines correspond to the different size classes (see text), and the thick lines represent the ensemble mean for each of the three glaciers. The black dashed line indicates the overall ensemble mean, and dotted lines represent one standard deviation around this mean.
